# Supplementary material for: High-performance source of indistinguishable polarization-entangled photons with a local oscillator reference for quantum networking
Source: arXiv:2602.10317 source file (2026-04-14)
Supplement: Supplementary file 1 [file supplement_v3.pdf]

## 1. SECOND ORDER CORRELATION

Second-order correlation measurements $g^{(2)}(\tau)$ measure the degree of bunching $g^{(2)}(0) > 1$ or anti-bunching $g^{(2)}(0) < 1$ that an optical mode field has [1, 2]. The distribution of photon number states expected for a single mode of down-conversion is thermal, which has a $g^{(2)}(0) = 2$ [2, 3]. As multiple thermal modes are added, the $g^{(2)}(0)$ approaches 1 [2, 3]. This is due to the universality of the Poisson distribution for independent rate events [3]. $g^{(2)}(\tau)$ acts as a measurement of the number of modes a photon occupies and can be used to easily diagnose photon purity [3]. To measure $g^{(2)}(0)$, we use a Hanbury-Brown-Twiss interferometer triggered by our local oscillator. The output of the beam splitter in this setup can be used to estimate $g^{(2)}(0)$ [2].

$$g^{(2)}(0) \approx \frac{P_{cc}}{\sqrt{P_s P_i}} \approx 1 + 1/K \tag{S1}$$

where $P_{cc}$ is the probability of a coincidence per pump pulse, while $P_i$, $P_s$ are the probability of a signal and idler photon per pump pulse, respectively [2, 3].

We measure $g^{(2)}(0)$ using a 50:50 beam splitter on one of down-conversion modes. These photons are detected by two SNSPD detectors [2]. We verify that the photons are spectrally pure using time of flight spectroscopy, which allows us to use $g^{(2)}(0)$ to optimize the temporal width of the single photons by tuning the pulse compressor on the pump. First, we optimize the compression of the pump pulse using intensity autocorrelation. We then measure $g^{(2)}(0)$ of $1.977 \pm 0.001$. We observe that the $g^{(2)}(0)$ value depends on the bin size of the $g^{(2)}(0)$ measurement due to timing jitter of the detectors. A larger bin sizes capture more real counts, but also more dark counts. These dark counts bias the measurement to lower values as a coincidence from dark counts is unlikely. This measurement infers a temporal and spectral purity of $97.7 \pm 0.1\%$ in a bin size of 3 ns.

## 2. DUTY CYCLE APODIZATION OF SPDC CRYSTAL

To apodize our SPDC crystal we use duty cycle modulation similar to reports by Pickston et al. and Dixon et al. [4, 5]. A full derivation of the relationship between duty cycle and effective nonlinearity is given below allowing for arbitrary design using analytic functions. Changing the duty cycle away from 50% on/off in either direction reduces the effective nonlinearity. By changing the duty cycle along the propagation direction of the crystal we can construct an arbitrary effective nonlinearity curve for apodization.

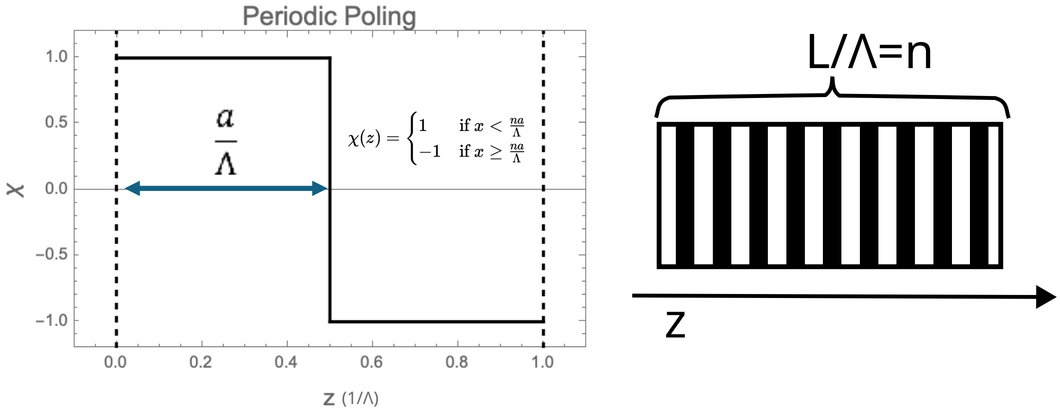


**Fig. S1.** A depiction of the poling profile that is being Fourier transformed with the relevant variables. This pattern is repeated $n$ integer times

The SPDC field ($E_{s,i}$) in the crystal can be calculated by integrating the pump field along the crystal. This integral is a Fourier transform making calculations of phase matching convenient.

$$\frac{\partial E_{s,i}}{\partial z} \propto \int \chi(z) \exp(i \Delta k z) dz \tag{S2}$$

$$\frac{\partial E_{s,i}}{\partial z} \propto \int_{L/2}^{L/2} \chi(z) \exp(i\Delta k z) dz \tag{S3}$$

The nonlinearity is a square wave with period $\Lambda = 1/L$ and some fraction of initial on distance $a \in [0, 1]$. This is then repeated at $n$ integer multiples. The apodization of nonlinearity in the crystal is controlled by the $a$ term.

$$\chi(z) = \begin{cases} 1 & \text{if } z < \frac{na}{\Lambda} \\ -1 & \text{if } z \geq \frac{na}{\Lambda} \end{cases} \tag{S4}$$

For the full derivation we can integrate over each of these poling regions

$$\frac{\partial E_{s,i}}{\partial z} \propto \int_{-L/2}^{-L/2+1/\Lambda} \chi(z) \exp(i\Delta k z) dz + \int_{-L/2+1/\Lambda}^{-L/2+2/\Lambda} \chi(z) \exp(i\Delta k z) dz + ... \tag{S5}$$

$$\propto \int_{0}^{a/\Lambda} \chi(z) \exp(i\Delta k z) dz + \int_{a/\Lambda}^{1/\Lambda} \chi(z) \exp(i\Delta k z) dz \tag{S6}$$

$$\propto \int_{0}^{a/\Lambda} 1 \exp(i\Delta k z) dz + \int_{a/\Lambda}^{1/\Lambda} -1 \exp(i\Delta k z) dz \tag{S7}$$

$$\propto \left. \frac{-i \exp(i\Delta k z)}{\Delta k} \right|_{0}^{a/\Lambda} + \left. \frac{\exp(i\Delta k z)}{\Delta k} \right|_{a/\Lambda}^{1/\Lambda} \tag{S8}$$

$$\propto \frac{i}{\Delta k} [(1 - \exp(i\Delta k a/\Lambda)) + (\exp(i\Delta k/\Lambda) - \exp(i\Delta k a/\Lambda))]. \tag{S9}$$

Simplifying using $\frac{2\pi}{\Delta k} = \frac{1}{\Lambda}$ we obtain

$$\frac{2i}{\Delta k} [1 - \exp(i2\pi a)], \tag{S10}$$

whose maximum is $\frac{2i}{\Delta k}$. We can normalize this to get the effective nonlinearity of

$$\chi_{eff} = \frac{1 - \exp(i2\pi a)}{2}. \tag{S11}$$

Taking the absolute square of this, we can calculate the intensity as a function of $a$:

$$\chi_{eff}^2 = \frac{2(1 - \cos(2\pi a))}{4}. \tag{S12}$$

Using a double angle formula, we can convert this to

$$\chi_{eff}^2 = \sin^2(\pi a) \tag{S13}$$

and finally

$$\chi_{eff} = \sin(\pi a). \tag{S14}$$

## 3. CRYSTAL MASK DESIGN

The crystal was commercially fabricated by lithographically fabricating poling electrodes defined by a 1 dimensional mask. When generating the crystal mask pattern used from these analytic functions it is convenient to have a the crystal poling be a continuous function of $z$. We can do this by taking the sign of some cosine function with an offset. This can be useful for generating the crystal poling on a Fourier grid without aliasing. The poling function can be defined as

$$\chi(z) = \text{sign}\Big( \cos\left(\frac{2\pi z}{L}\right) + d(z) \Big). \tag{S15}$$

Where $d(z)$ is the duty cycle modulation and the sign functions is positive 1 for positive arguments and $-1$ for negative arguments. The point at which the function will change signs, $\cos\left(\frac{2\pi z}{L}\right) + d(z) = 0$. For this function, the effective poling relationship is given by

$$\chi_{eff}(z) = \sqrt{1 - d(z)^2} \tag{S16}$$

The mask was calculated using the online program SPDCalc developed by our group [6].

## 4. MONOLITHIC MOUNT

We generate polarization entanglement by pumping two spatially separate modes of the nonlinear crystal and erasing the which-path information between photons generated in either mode [7–9]. This process results in the entangled polarization state

$$|\psi\rangle = \frac{1}{\sqrt{2}}(|HV\rangle + e^{i\phi}|VH\rangle). \quad \text{(S17)}$$

where the relative phase $\phi$ depends on the path length of the two pump modes in the interferometer [7–9]. First, we rotate the pump to diagonal polarization using a half waveplate (HWP) at 22.5 degrees. Then the pump is passed through an alpha barium borate 2 mm offset polarizing beam displacer. Next, we rotate the horizontal mode (which does not experience an offset) to vertical. The spatially separated pump modes both undergo a type-II down-conversion process in the crystal. We use a vertical beam displacer to separate the H and V photons into a total of four modes. We use a diced HWP to rotate the polarizations of the down-converted light in the horizontally offset modes. We use a pick-off mirror to separate the pairs of vertically offset modes from each other. Finally in each pair of modes we use a horizontal beam displacer to recombine the paths into a single mode. We built the entire polarization Mach-Zehnder interferometer on a custom manufactured aluminum mount, which was measured to have a passive polarization alignment with 97,000:1 ± 2,000:1 extinction between polarization modes.

## 5. CHIRP PULSE AMPLIFICATION

The pulse is expanded in time using a multi-pass Martinez expander [10, 11]. Light enters and exits the expander through a fiber circulator, which separates the input pulse from the expanded and filtered output. The Martinez stretcher uses four passes through a 1000 grooves/mm grating with 52 degree incidence and 20 cm lens, which is de-focused by $(12.7 \pm 0.4)$ cm providing a total of $(14.4 \pm 0.6)$ $ps^2$ of dispersion. The pulse is filtered using a tunable slit aperture after its frequencies are spatially dispersed by the grating. The expander produces a $(5.42 \pm 0.03)$ nm bandwidth pulse with a total efficiency of $(8.9 \pm 0.2)$%. This is then amplified using a commercial erbium doped fiber amplifier (EDFA) to $(551.5 \pm 0.2)$ mW. We minimize the fiber length at the output of the EDFA to prevent nonlinearities. We then recompress the pulse using a four pass free space Treacy compressor, which has a tunable dispersion [12, 13]. This produces a $(1.37 \pm 0.02)$ ps duration pulse with a $(3.16 \pm 0.03)$ nm bandwidth at $(362.8 \pm 0.5)$ mW average power. Finally, we focus this pulse into a 5 mm (MgO:ppLN) crystal that is 3 mm long with a 19.2 $\mu m$ poling period that is heated to 70 $^oC$. This SHG process produces a $(0.608 \pm 0.006)$ nm bandwidth 775 nm pulse at an average power of $(67 \pm 2)$ mW

## 6. COLLECTION INTO FIBER

We collect the light using 15 cm lenses into a collimated beam, which is then focused into a commercial GRIN fiber coupler using a 40 cm lens. These GRIN fibers produce a $(0.190 \pm 0.004)$ mm spot at $(7.5 \pm 0.5)$ mm. We ensure that at least two mirrors are used between the fiber and Mach-Zehnder to allow control over all degrees of freedom. We fold both lens systems using 99.99% reflectivity dielectric folding mirrors. After efficiently collecting the photons into fiber, we detect them using in-house fabricated superconducting nanowire single-photon detectors (SNSPD) optimized for high efficiency at 1550 nm. These include a Bragg reflector and anti-reflective (AR) coating optimized for 1550 nm [14]. These detectors are not matched with an adiabatic taper and are large area, giving them a high timing jitter $(223 \pm 2)$ ps FWHM. Additionally, due to the large area, the dead time is $(309 \pm 6)$ ns at $1/e$ count rate. This is when the rate of consecutive clicks reaches $1/e$ if its maximum as a function of delay. We measured the SDE of the four detectors to be $(93.4 \pm 0.4)$%, $(96.3 \pm 0.5)$%, $(92.8 \pm 0.4)$%, $(93.4 \pm 0.5)$%. We measured these at rate of $(100,000 \pm 300)$ counts per second. We record the output voltage pulses from these nanowires using a commercial time tagger with a 5 ps timing jitter, an 80 ns dead time. The dead-time was set deliberately large to prevent re-triggering. We determined the bias of detectors using system detection efficiency curves; we used the bias current which yielded unity internal efficiency. We set the time tagger trigger threshold by minimizing jitter.

## 7. HONG-OU-MANDEL INTERFEROMETRY

We interfere two idler photons by sending the signal photons onto a beam splitter, with one path going through a 10 ns delay before entering the HOM setup and the other going straight in. We

combine these two paths on a polarizing beam splitter, one of which is reflected towards the second PBS. The other we pass through a circulator with tunable delay formed by the PBS and a QWP. We then combine these two modes through a HWP to tune the PBS splitting ratio. Finally, we precompensate the fiber polarization rotation using a QWP and HWP. To align the pulses in time We first perform a rough alignment by cutting a delay fiber to the correct length, given the path difference of the two arms, which we measure using the time taggers. We use a single-source HOM to optimize our measurement system to ensure high visibilities are measurable. In this case we send a signal and idler into the HOM interferometer and tune the delay.

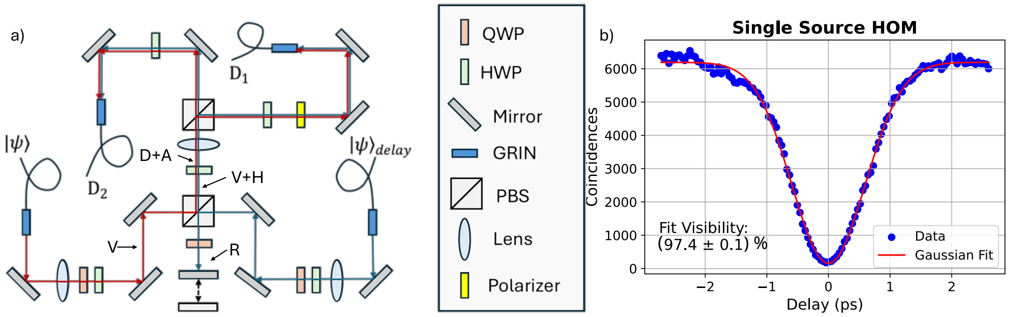


**Fig. S2.** a) A depiction of the setup used for HOM interferometry. b) a plot of the measured single source HOM dip, where we interfere the signal and idler produced by the same pulse

To calculate the visibility in power dependent measurements first, we took a full HOM dip at high power. Then, for each power, we collected the rate of four-fold coincidences at two delays determined by the first measurement: zero delay (dip minimum) and long delay (baseline). This significantly reduced the time required for power-dependent measurements, allowing us to feedback on the interference visibility by tuning the pump laser spectrum and pulse compression. However, we observed this process to produce lower estimates in visibility, due a shift of the delay location for the minimum of the dip. The dip delay corresponding to the minimum was observed independently to have a standard deviation of $(0.05 \pm 0.02)$ ps which is about $(3 \pm 1)\%$ of the FWHM. Because the coincidence rate is significantly lower at the dip minimum than on the long-delay baseline, we collected the four fold coincidences at the dip minimum for three times longer than the baseline. We calculate this as the optimal collection time ratio to maximize the uncertainty reduction per coincidence for an anticipated 95% dip visibility.

## 8. PURITY AND THE HOM DIP

The HOM dip is a quantum optical measurement used as a quantitative estimate of the purity of a state[15, 16]. Previous work has shown that the HOM dip visibility of two separable states is equal to the purity [15, 16]. This is only true for states with low photon numbers. In our experiment we experience a non-negligible reduction in measured purity due to higher order photon events. Previous work has demonstrated that a linear fit is sufficient to extrapolate what the purity would be assuming one has perfect number-resolving detectors or low photon numbers[5, 17].

In our work we use a heralding detector which was quasi-number resolving. This necessarily induces nonlinearities in the power dependence of the measured HOM visibility which may be non-negligible. In the following sections, we prove that the function governing the power dependence of the visibility is linear within the operating parameters of our experiment despite the number resolving herald. This allows us to perform a linear fit to extrapolate the purity of our state assuming a perfect number-resolving herald. Instead of brute forcing the boson counting problem we follow the following plan. We first calculate the visibility of the HOM dip for input modes consisting of $n$ and $m$ indistinguishable photons. We then project the two mode squeezed vacuum state using a number resolving herald to determine the state input into the HOM interferometer. Finally we calculate the power dependence of the HOM visibility for low pump powers, and estimate the accuracy of the linear assumption in our fits.

### A. HOM Visibility

Previous work, [15, 16], has shown for a mixed state the HOM dip visibility is

$$V_0 = Tr[\rho_a \rho_b], \tag{S18}$$

Where $\rho_a$ and $\rho_b$ are density matricies of the input modes. This is valid for a two state system, but breaks down for higher dimensional systems. For example, the purity of a maximally mixed photon number state of dimension $d$ will be $1/d$.

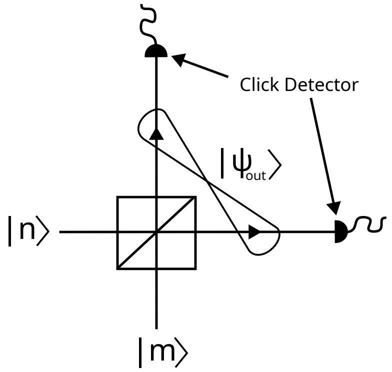


**Fig. S3.** a) A depiction of the interference occurring on a beam splitter whose output state is measured on click detectors. These measure 1 or more photons as a click. The coincidences of indistinguishable vs. distinguishable photons are used to calculate visibility. Distinguishability is tuned through delay

We can calculate the maximum visibility of the HOM using the general equations of two photon number states, $|n\rangle$ and $|m\rangle$ incident on a beam splitter. For the maximum coincidences the probability of no coincidence will be simply the probability that $n+m$ photons go into a single mode. We can then subtract this from one to obtain the probability of a coincidence

$$P_c^{max} = 1 - \frac{1}{2^{n+m-1}} \tag{S19}$$

For the minimum of the dip we can calculate the coincidence probability using the resulting state from indistinguishable photon number states on a beam splitter. The resulting state output state from $|n\rangle$ in one port and $|m\rangle$ in another is given by [18]

$$|\psi_{out}\rangle = \sum_{k=0}^{n+m} \sqrt{\frac{n!\,m!}{k!\,(n+m-k)!}} \frac{1}{2^{\frac{n+m}{2}}} \sum_{j=0}^{n} (-1)^{n-j} \binom{n}{j} \binom{m}{k-j} |k\rangle |n+m-k\rangle \tag{S20}$$

For no coincidence we have no photon in one of the outputs, either $k=0$ or $k=n+m$. In this case we have

$$|\psi_{out}\rangle = \sqrt{\frac{n!m!}{(n+m)!}} \frac{1}{2^{\frac{n+m}{2}}} \sum_{j=0}^{n} (-1)^{n-j} \binom{n}{j} \binom{m}{-j} |0\rangle |n+m\rangle \tag{S21}$$

We can use Vandermode's identity

$$\sum_{j=0}^{\infty} (-1)^{n-j} \binom{n}{j} \binom{m}{r-j} = (-1)^n \binom{m-n}{r-n}. \tag{S22}$$

Setting $r=0$, we obtain

$$|\psi_{out}\rangle = \sqrt{\frac{n!m!}{(n+m)!}} \frac{1}{2^{\frac{n+m}{2}}} (-1)^n \binom{n-m}{0-n} |0\rangle |n+m\rangle. \tag{S23}$$

For the probability that $k=0$ we have

$$\left[ \sqrt{\frac{n!m!}{(n+m)!}} \frac{1}{2^{\frac{n+m}{2}}} (-1)^n \binom{n-m}{0-n} \right], \tag{S24}$$

Which can be converted to a regular binomial index through the generalized binomial coefficient:

$$P_{k=0} = \left[ \sqrt{\frac{n!m!}{(n+m)!}} \frac{1}{2^{\frac{n+m}{2}}} \binom{n+m}{n} \right]^2 \tag{S25}$$

. Taking the square we obtain

$$P_{k=0} = \frac{n!m!}{(n+m)!}\frac{1}{2^{n+m}}\binom{n+m}{n}^2 \tag{S26}$$

The first term is equal to the inverse of the binomial coefficient $\binom{n+m}{n}$. Finally we have two cases of no coincidences with this factor, so the probability of coincidences is

$$P_c^{min} = 1 - 2P_{k=0} = 1 - \frac{1}{2^{n+m-1}}\binom{n+m}{n} \tag{S27}$$

Finally we can calculate the visibility by $V = (P_c^{max} - P_c^{min})/P_c^{max}$. Simplifying we obtain the final equation of

$$V(n,m) = \frac{\binom{m+n}{m} - 1}{(2^{m+n-1} - 1)} \tag{S28}$$

For the $|11\rangle$ state we have the regular value of 1, the next most relevant term is the 2, 1 term which gives 2/3. This factor modifies the expected dependence of visibility on pump power. In general we can look at high dimensional photon number state mixtures that are produced by heralding a photon on a click detector. This will result in a purity measurement modulated by the photon number state. We can treat the visibility as an observable on the density matrix. The heralded state of a click detector is

$$\rho_n = 1/Z_n \sum_{n=1}^{\infty} a_n |n\rangle\langle n| \tag{S29}$$

$$\rho_m = 1/Z_m \sum_{m=1}^{\infty} a_m |m\rangle\langle m| \tag{S30}$$

When the HOM dip occurs the visibility will be modulated by a factor of $V(n,m)$ depending on which photon number state occurs. The expected value of the visibility will be

$$V = \sum_{n=1}^{\infty}\sum_{m=1}^{\infty} a_n b_m \frac{\binom{n+m}{m} - 1}{(2^{n+m-1} - 1)} \tag{S31}$$

in general we herald the same state which will depend on $\lambda^n$ so we can look at total photon number $k = m + n$. Now that we can calculate the visibility for particular photon number states we can move on to estimating the mixture that our source produces.

### B. Number Resolving Herald

In this section, we will use projection operators to calculate the state our source heralds. In previous experiments consecutive photons are heralded using the same detector and a long delay line (approximately 100 ns). Our detectors have such a large dead time that a delay line would introduce significant dispersion. We instead utilize two SNSPDS in a pseudo-number resolving configuration and a 10 ns delay line. Each detector detects a single herald from each pulse while filtering multi-pair events. The idler states produced by the down-conversion are incident on a beam splitter and detected by two click detectors. If a given pulse generates 2 clicks in either the early or late bin, we disregard that trial. We depict the two configurations we will analyze with the relevant variables in Fig. S4.

First we will assume that the purity of the state in the number basis is independent of the spectral temporal basis such that

$$\rho = \rho_{\omega\tau} \otimes \rho_n \tag{S32}$$

Which means the purity can be decomposed into a product

$$Tr[\rho^2] = Tr[\rho_{\omega\tau}^2]Tr[\rho_n^2] \tag{S33}$$

The purity of the resulting state in the number bases, from a heralding detector can be determined from the resulting projection of the detectors positive operator valued (POVM) measurement [19]. The state generated in SPDC can be described as a two mode squeezed vacuum:

$$|\psi\rangle = \sqrt{1 - |\lambda|^2}\sum_{n=0}^{\infty} \lambda^n |n_s n_i\rangle . \tag{S34}$$

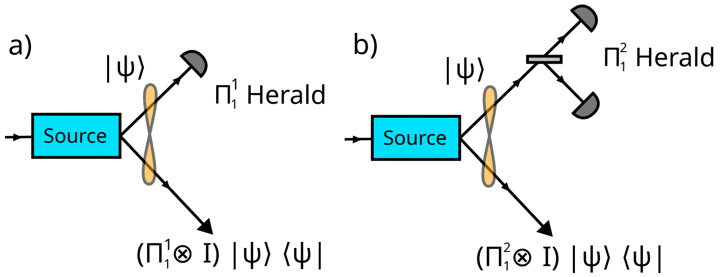


**Fig. S4.** A depiction of the two heralded SPDC configurations we are considering and the relevant states and operators. a) A click detector which detects 1 or more photons heralding a SPDC source. b) A two mode pseudo number resolving click detector heralding an SPDC source.

The POVM of an arbitrary photon number state detector is

$$\Pi = \sum_{n=0}^{\infty} c_n |n\rangle \langle n| . \tag{S35}$$

These can be combined to calculate the non-normalized heralded state via

$$(\Pi \otimes I) |\psi\rangle \langle\psi| = \rho_n = \frac{1}{N^2} \sum_{n=0}^{\infty} c_n^2 \lambda^{2n} |n\rangle \langle n| \tag{S36}$$

which must be normalized by finding the convergence of the sum

$$N^2 = \sum_{n=0}^{\infty} c_n^2 \lambda^{2n} |n\rangle \langle n| . \tag{S37}$$

We will consider the following POVM operators for Eq. S35, each of which converge for detector efficiency $0 < \eta < 1$. The general form of these equations can be found in [19]. For the single-mode detector with one click we have

$$\Pi_1^1 = \sum_{n=0}^{\infty} [(1-(1-\eta)^n] |n\rangle \langle n| \tag{S38}$$

and for the two-mode detector with one click we have

$$\Pi_1^2 = \sum_{n=0}^{\infty} [2((1-\eta/2)^n - (1-\eta)^n)] |n\rangle \langle n| \tag{S39}$$

These two POVM result in a convergence of the infinite sum to the following analytic expressions of purity. The purity and normalization equations are found by expanding the $c_n$ terms, then equating terms to the geometric series. For the single-mode detector we obtain.

$$N^2(\Pi_1^1) = -\frac{2}{1-(1-\eta)\lambda^2} + \frac{1}{1-(1-\eta)^2\lambda^2} + \frac{1}{1-\lambda^2} \tag{S40}$$

and for the two-mode detector with one click (the herald we use in out experiment) we obtain

$$N^2(\Pi_1^2) = -\frac{8}{1-\left(1-\frac{\eta}{2}\right)(1-\eta)\lambda^2} + \frac{4}{1-(1-\eta)^2\lambda^2} + \frac{4}{1-\left(1-\frac{\eta}{2}\right)^2\lambda^2} \tag{S41}$$

These give the resulting state produce by heralding the output of a SPDC source with both a regular click detector, and a two mode pseudo number resolving click detector. These states represent mixtures in the photon number basis which can be combined with out visibility equation to determine the resulting visibility at a particular pump power.

### C. Power Dependent Visibility

We will now calculate the power dependence of the visibility for both cases outlined in the previous subsection: a single click detector, and a pseudo number resolving click detector with two modes. For either detector case we have the general form from Eq. S36

$$\frac{1}{N^2}\sum_{n=0}^{\infty} c_n^2 \lambda^{2n} |n\rangle \langle n| \tag{S42}$$

Which in the visibility Eq. S31 will become

$$V = \frac{1}{N^4}\sum_{n=0}^{\infty}\sum_{m=0}^{\infty} c_n^2\lambda^{2n}c_m^2\lambda^{2m}\frac{\binom{n+m}{m}-1}{(2^{n+m-1}-1)} \tag{S43}$$

The correction this makes to the purities in the previous proof will depend on the order of squeezing that is relevant. For a squeezing of $\lambda^2$ we obtain the correction

$$V_{\Pi_1^1} = 2P(1)P(2)V(1,2) + P(1)^2V(1,1) + O[\lambda^3] \tag{S44}$$

This is the dominant correction for our experiment. Additionally the pump power $P$ and measured coincidence probability per pulse $\mu$ on a click detector is related to squeezing through

$$\lambda = \text{Tanh}[a\sqrt{P}] = \sqrt{\frac{\mu}{\eta}}, \tag{S45}$$

The coincidence probability per pulse $\mu$ is the measured coincidence rate divided by the measured repetition rate of the pump. This results in the visibility

$$V_{\Pi_1^1} \approx 1 - \frac{2}{3}(\eta-2)^2\frac{\mu}{\eta} + O[\mu^3]. \tag{S46}$$

Similarly for the pseudo number resolving visibility we obtain

$$V_{\Pi_1^2} \approx 1 - \frac{1}{6}(3\eta-4)^2\frac{\mu}{\eta} + O[\mu^3], \tag{S47}$$

which for $\eta \to 1$ and $\mu \to 0$ are both linear. Additionally the visibility curve is concave up meaning a linear fit will underestimate the visibility. Using detector efficiency and $n \geq 1$ per pulse probability from our experiment, the error of the linear approximation is on order of $10^{-4}$. This is well below the uncertainty of our measurement, which has a fractional uncertainty of approximately $6 \times 10^{-3}$.

## 9. LOCAL-OSCILLATOR SINGLE-PHOTON HOM

The spectral-temporal dependence of this HOM dip is the same as the successive photon dip. To obtain a high visibility the heralded photons must be pure. Therefore, we will only look at the dependence on the intensity of the coherent state. This process is depicted below

Ignoring the spectrum of the single photon and coherent state, the input state is

$$|\psi_{\text{in}}\rangle = |1\rangle \otimes |\alpha\rangle \tag{S48}$$

After going through the beam splitter, the resulting state is

$$|\psi_{\text{out}}\rangle = (t\hat{a}^\dagger \otimes I + I \otimes r\hat{b}^\dagger)(|r\alpha\rangle \otimes |-t\alpha\rangle) \tag{S49}$$

Assuming perfect click detector efficiency, the coincidence probability can be calculated via

$$P_{11} = 1 - P_{a0} - P_{0b} + P_{00} \tag{S50}$$

This case always has a photon leaving a port, meaning $P_{00} = 0$.

Here, $P_{11}$ represents the probability of there being "not 0" photons in each mode. In the limit of 100% efficiency, $P_{11}$ is equivalent to the measured coincidence rate.

To find $P_{a0}$, we project onto the state:

$$(I_a \otimes |0\rangle\langle 0|)|\psi_{\text{out}}\rangle = |\psi_a\rangle \tag{S51}$$

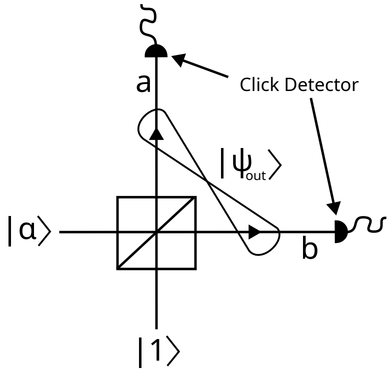


**Fig. S5.** A depiction of the interference occurring on a beam splitter of a coherent state and single photon into the output modes a and b.

Looking at $|\psi_{\text{out}}\rangle$, the $\hat{b}^\dagger$ term negates the contribution of $\langle 0|$ acting on it, and the only term left is

$$t\hat{a}^\dagger|r\alpha\rangle \otimes |0\rangle \tag{S52}$$

The magnitude of this then gives the $P_{a0}$ contribution:

$$P_{a0} = \langle r\alpha||t|^2\hat{a}\hat{a}^\dagger|r\alpha\rangle \cdot |\langle 0| - t\alpha\rangle|^2 \tag{S53}$$

Using $\hat{a}^\dagger\hat{a} = \hat{n}$ and $[\hat{a}, \hat{a}^\dagger] = 1 \Rightarrow \hat{a}\hat{a}^\dagger = 1 + \hat{n}$, we have

$$P_{a0} = |t|^2(1 + |r\alpha|^2)e^{-|t\alpha|^2} \tag{S54}$$

Similarly,

$$P_{0b} = |r|^2(1 + |t\alpha|^2)e^{-|r\alpha|^2} \tag{S55}$$

And the coincidences are:

$$P_{11} = 1 - |t|^2(1 + |r\alpha|^2)e^{-|t\alpha|^2} - |r|^2(1 + |t\alpha|^2)e^{-|r\alpha|^2} \tag{S56}$$

As a function of coherent state amplitude, the visibility is calculated with

$$V = \frac{P_{11,\text{max}} - P_{11,\text{min}}}{P_{11,\text{max}}} \tag{S57}$$

The visibility as a function of coherent state $\alpha$ with a perfect single photon is then

$$V = \frac{(2 + \alpha^2)e^{\alpha^2/2} - 2}{2(e^{\alpha^2} - 1)} \tag{S58}$$

For a maximum visibility of 99.9%, the coherent state amplitude must be $\alpha = 0.09$. A derivation following the previous section on HOM visibility in the number state basis yields the same result. This function as derived does not approach 1/2, which is the standard classical limit.

## REFERENCES


1. T. J. Bartley, G. Donati, J. B. Spring, *et al.*, "Multiphoton state engineering by heralded interference between single photons and coherent states," Phys. Rev. A **86**, 043820 (2012).
2. M. J. Stevens, "Chapter 2 - photon statistics, measurements, and measurements tools," in *Experimental Methods in the Physical Sciences,* vol. 45 of *Single-Photon Generation and Detection* A. Migdall, S. V. Polyakov, J. Fan, and J. C. Bienfang, eds. (Academic Press, 2013), pp. 25–68.
3. N. Bruno, A. Martin, and R. T. Thew, "Generation of tunable wavelength coherent states and heralded single photons for quantum optics applications," Opt. Commun. **327**, 17–21 (2014).
4. P. B. Dixon, J. H. Shapiro, and F. N. C. Wong, "Spectral engineering by gaussian phase-matching for quantum photonics," Opt. Express **21**, 5879–5890 (2013).
5. A. Pickston, F. Graffitti, P. Barrow, *et al.*, "Optimised domain-engineered crystals for pure telecom photon sources," Opt. Express **29**, 6991–7002 (2021).

6. L. K. Shalm, "Spdcalc," http://spdcalc.org/ (2022).
7. L. K. Shalm, Y. Zhang, J. C. Bienfang, *et al.*, "Device-independent randomness expansion with entangled photons," Nat. Phys. **17**, 452–456 (2021).
8. L. K. Shalm, E. Meyer-Scott, B. G. Christensen, *et al.*, "Strong loophole-free test of local realism," Phys. Rev. Lett. **115**, 250402 (2015).
9. C. Zhang, Y.-F. Huang, B.-H. Liu, *et al.*, "Spontaneous parametric down-conversion sources for multiphoton experiments," Adv. Quantum Technol. **4**, 2000132 (2021).
10. O. E. Martinez, "Grating and prism compressors in the case of finite beam size," JOSA B **3**, 929–934 (1986).
11. A. Ruiz-de-la-Cruz and R. Rangel-Rojo, "Multi-pass confocal ultra-short pulse amplifier," Revista mexicana de física **51**, 488–493 (2005).
12. V. Chauhan, P. Bowlan, J. Cohen, and R. Trebino, "Single-diffraction-grating and grism pulse compressors," JOSA B **27**, 619–624 (2010).
13. Z. Zhong, W. Gong, H. Jiang, *et al.*, "Investigation of spatial chirp induced by misalignments in a parallel grating pair pulse stretcher," Appl. Sci. **10**, 1584 (2020).
14. D. V. Reddy, R. R. Nerem, S. W. Nam, *et al.*, "Superconducting nanowire single-photon detectors with 98% system detection efficiency at 1550 nm," Optica **7**, 1649–1653 (2020).
15. A. M. Brańczyk, "Hong-ou-mandel interference," (2017).
16. J. C. Garcia-Escartin and P. Chamorro-Posada, "swap test and hong-ou-mandel effect are equivalent," Phys. Rev. A **87**, 052330 (2013).
17. F. Graffitti, P. Barrow, M. Proietti, *et al.*, "Independent high-purity photons created in domain-engineered crystals," Optica **5**, 514–517 (2018).
18. R. A. Campos, B. E. A. Saleh, and M. C. Teich, "Quantum-mechanical lossless beam splitter: Su(2) symmetry and photon statistics," Phys. Rev. A **40**, 1371–1384 (1989).
19. S. Sempere-Llagostera, G. S. Thekkadath, R. B. Patel, *et al.*, "Reducing $g^{(2)}(0)$ of a parametric down-conversion source via photon-number resolution with superconducting nanowire detectors," Opt. Express **30**, 3138–3147 (2022).
